# Supplementary material for: Safe and Efficient Model Predictive Control Using Neural Networks: An Interior Point Approach
Source: arXiv:2203.12196 source file (2022-09-13)
Supplement: Supplementary file 1 [file 6_appendix.tex]

\appendix

Below, we construct an affine function $\phi$ that returns an interior point of $\V(x)$ for all $x \in \X$, if such a function exists. Let $\phi(x) = Wx + w$. The criteria on $(W,w)$ are \begin{align}
    F_x(Ax + B(Wx+w)) < \tilde{g}_x,\ F_u u < g_u \ \forall\ x \in \X. \label{eqn:2-28-1}
\end{align}

Let $\Y(s) = \{x \in \R^n \mid F_x(Ax + B(Wx+w)) \leq \tilde{g}_x + s \textbf{1},\ F_u u \leq g_u + s\textbf{1}\}$. The criteria in \eqref{eqn:2-28-1} are restated as \begin{align}
    \X \subseteq \Y(s) \text{ for some } s < 0.
\end{align} The condition $\X \subseteq \Y(s)$ is a polytope containment criterion \todo{cite} which can be posed as a set of linear equality and inequality constraints on $W$ and $w$. To choose the parameters $W$ and $w$, we solve the following linear program: \begin{subequations} \begin{gather}
    \min_{W,w,s} s \\
    \text{subject to: } \X \subseteq \Y(s).
\end{gather} \end{subequations} If the optimal cost is less than 0, then an affine solution to finding an interior point of $\V(x)$ for all $x \in \X$ exists and is given by $\phi(x) = Wx + w.$
